# Supplementary material for: Distributed Deep Joint Source-Channel Coding over a Multiple Access Channel
Source: arXiv:2211.09920 source file (2023-03-02)
Supplement: Supplementary file 1 [file appendix.tex]

\appendix

\subsection{Analysis of Wireless Conditions}
\label{sec:tab_channel_conditions}
% Please add the following required packages to your document preamble:
% \usepackage{booktabs}
\begin{table*}[!tbp]
\caption{Comparison of methods in terms of wireless channel conditions for two-user case}
\label{tab:channel_conditions_comparison}
\centering
\begin{tabular}{@{}lcccc@{}}
\toprule
Method        & Noise Variance & Average Power per Bandwidth & Bandwidth per User & Total Power per User \\ \midrule
DeepJSCC-TDMA & $\sigma^2$ & $2\Pavg$                         & k/2                & $k\Pavg$                           \\
DeepJSCC-NOMA  & $\sigma^2$ & $\Pavg$                          & k                  & $k\Pavg$ \\
\bottomrule
\end{tabular}
\end{table*}
For clarity, Table~\ref{tab:channel_conditions_comparison} shows the analysis of channel conditions and constraints for the compared methods. The total power per user, which is half of the total power used, must be equal for both methods to ensure fairness~\cite{tse2005fundamentals}.

%\subsection{Comparison with Digital Methods}
%\input{figures/deneme}

\subsection{NN Architecture}
\label{sec:nn_architecture}
\begin{table*}[!tp]
\centering
\caption{Detailed \gls{NN} architecture of the employed encoder and decoder}
\label{tab:nn_architecture}
\begingroup
 % Default value: 1
\begin{tabular}{lll}
\toprule
Component                & Layer                                   & Output Shape                     \\ \midrule
Encoder $i=1,2$ (at Tx1 and Tx2) & Input $\Tilde{\xv}_{i,t} = \begin{bmatrix} \xv_{i,t} & \rv_i \end{bmatrix}^T$                & $4 \times W \times H$            \\
                         & Residual Block Downsample ($s=2,N=256$) & $256 \times \frac{W}{2} \times \frac{H}{2}$      \\
                         & AF Module                               & $256 \times \frac{W}{2} \times \frac{H}{2}$      \\
                         & Residual Block ($N=256$)                & $256 \times \frac{W}{2} \times \frac{H}{2}$      \\
                         & Residual Block ($N=256$)                & $256 \times \frac{W}{2} \times \frac{H}{2}$      \\
                         & AF Module                               & $256 \times \frac{W}{2} \times \frac{H}{2}$      \\
                         & Attention Module                        & $256 \times \frac{W}{2} \times \frac{H}{2}$      \\
                         & AF Module                               & $256 \times \frac{W}{2} \times \frac{H}{2}$      \\
                         & Residual Block ($N=256$)                & $256 \times \frac{W}{2} \times \frac{H}{2}$      \\
                         & Residual Block Downsample ($s=2,N=256$) & $256 \times W/4 \times H/4$      \\
                         & AF Module                               & $256 \times W/4 \times H/4$      \\
                         & Residual Block ($s=1,N=\frac{64k}{WH}$)       & $\frac{64k}{WH} \times W/4 \times H/4$ \\
                         & AF Module                               & $\frac{64k}{WH} \times W/4 \times H/4$ \\
                         & Attention Module                        & $\frac{64k}{WH} \times W/4 \times H/4$ \\
%                         & Precoding                               & $\frac{64k}{WH} \times W/4 \times H/4$ \\
                         & Power Normalization                     & $\frac{64k}{WH} \times W/4 \times H/4$ \\ \midrule
\gls{MAC}                & Sum Pooling and Noise Addition          & $\frac{64k}{WH} \times W/4 \times H/4$ \\ \midrule
Decoder at Rx            & Attention Module                        & $\frac{64k}{WH} \times W/4 \times H/4$ \\
                         & Residual Block ($N=256$)                & $\frac{64k}{WH} \times W/4 \times H/4$ \\
                         & Residual Block ($N=256$)                & $\frac{64k}{WH} \times W/4 \times H/4$ \\
                         & AF Module                               & $\frac{64k}{WH} \times W/4 \times H/4$ \\
                         & Residual Block ($N=256$)                & $\frac{64k}{WH} \times W/4 \times H/4$ \\
                         & Residual Block Upsample ($s=2,N=256$)   & $\frac{64k}{WH} \times \frac{W}{2} \times \frac{H}{2}$ \\
                         & AF Module                               & $\frac{64k}{WH} \times \frac{W}{2} \times \frac{H}{2}$ \\
                         & Residual Block ($N=256$)                & $\frac{64k}{WH} \times \frac{W}{2} \times \frac{H}{2}$ \\
                         & Residual Block ($N=256$)                & $\frac{64k}{WH} \times \frac{W}{2} \times \frac{H}{2}$ \\
                         & AF Module                               & $\frac{64k}{WH} \times \frac{W}{2} \times \frac{H}{2}$ \\
                         & Residual Block ($N=256$)                & $\frac{64k}{WH} \times \frac{W}{2} \times \frac{H}{2}$ \\
                         & Residual Block Upsample ($s=2,N=6$)     & $6 \times W \times H$            \\
                         & AF Module                               & $6 \times W \times H$            \\
                         & Output Images $\begin{bmatrix} \hat{\vec{x}}_{1,t} & \hat{\vec{x}}_{2,t} \end{bmatrix}^T$ & $2 \times 3 \times W \times H$   \\ \bottomrule
\end{tabular}
\endgroup
\end{table*}
Table~\ref{tab:nn_architecture} details the neural network as the encoder and decoder of our method described in Section~\ref{sec:methodology}.
